# Supplementary material for: Non-simple flow behavior in a polar van der Waals liquid: structural relaxation under scope
Source: arXiv:2210.01947 source file (2022-10-04)
Supplement: Supplementary file 1 [file SI_Arrese-Igor.pdf]

# Supporting information:
# Non-simple mechanical response in a polar Van der Waals glass forming liquid: structural relaxation under scope

S. Arrese-Igor,[1] A. Alegría,[1, 2] and J. Colmenero[1, 2, 3]

[1]*Centro de de Física de Materiales (MPC), Centro Mixto CSIC-UPV/EHU, Paseo Manuel Lardizabal 5, 20018 San Sebastián, Spain*

[2]*Departamento de Física de Materiales UPV/EHU, Apartado 1072, 20080 San Sebastián, Spain*

[3]*Donostia International Physics Center, Paseo Manuel Lardizabal 4, 20018 San Sebastián, Spain*

(Dated: September 28, 2022)

## I. EXPERIMENTAL

TBP and ortotertphenyl (OTP) -used here as a reference sample for non polar van der Waals liquid- were purchased from Aldrich and stored with activated molecular sieves in order to eliminate traces of ionic impurities which could be present in the commercial products.

Possible differences between the thermocouple reading temperatures of each instrument for a given set point were evaluated by introducing the same thermocouple in both instruments. The temperature shift between different instruments was determined to be constant in the whole temperature range tested (between 120K and 340K) and equal to 0,2K.

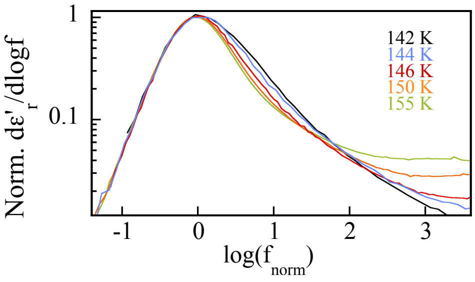


FIG. 1: Absolute value of the derivative of the real part of the permittivity.

### A. Dielectric Response

Isothermal broad band dielectric spectroscopy (BDS) experiments were carried out on a commercial Novocontrol Alpha A set-up where the temperature was controlled by a nitrogen-jet stream with a temperature stability of 0.1 K. Samples were sandwiched between two parallel gold-plated electrodes using Teflon thin strips as a spacer in a specific liquid cell. Results were corrected from stray capacitance of the cell and area of the Teflon strips. In addition to the usual magnitudes $\epsilon'(\omega)$ and $\epsilon''(\omega)$ (where $\epsilon^*(\omega) = \epsilon'(\omega) - i\epsilon''(\omega)$), data was also represented as the logarithmic frequency derivative of the real part of the permittivity $-d\epsilon'/d(log\omega)$. Derivative

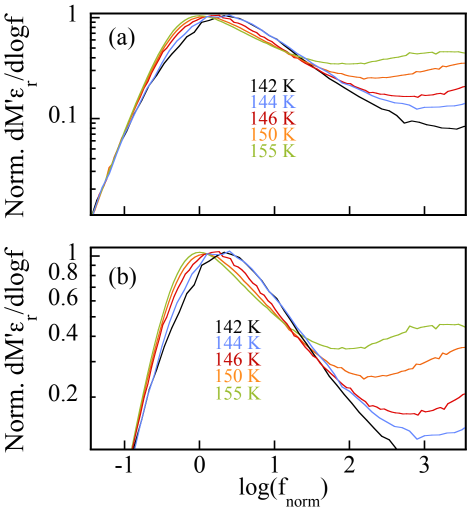


FIG. 2: Derivative of the real part of the electric modulus

representation of $\epsilon'(\omega)$ data eliminates dc-conductivity and might aid in resolving overlapped processes as they show as narrower peaks than in $\epsilon''(\omega)$.

Analysis of the evolution of the dielectric signal with temperature shows that the lineshape of the main peak is not constant. Figures S1 and S2 represent dielectric data as a function of frequency at different temperatures. In figure S1 we represent the absolute value of the derivative of the real part of the permittivity and in figure S2 the derivative of the real part of the electric modulus. In all these figures data in the $y$-axis were normalized to maxima values. The frequency axis on the other hand was normalized (shifted in the logarithmic scale) so that the low frequency wing of the curves at different temperatures match together taking as a reference the curve at 155K. For permittivity lineshape only changes at the hight frequency wing whereas it changes both above and below the maxima position in modulus representation. Taking into account the observed lineshape evolution and that the relative weight of different processes changes among these two representations, this behavior is consistent with the presence of two overlapping contributions where the relative separation between the two components changes with temperature and be-

comes smaller the lower the temperature.

### B. Shear Response

The oscillatory shear response was measured by means of a TA Instruments ARES rheometer with a separate motor transducer using invar plates (8 mm diameter) in parallel geometry. The temperature of the sample was controlled by an long arm oven set-up under nitrogen flow with a temperature stability of 0.02 K. Dynamic strain sweep tests were performed at high frequency to determine the linear regime in which the storage ($G'$) and loss ($G''$) moduli were constant and strain in this linear regime was chosen for subsequent measurements which provide torque in the desired range. Shear data was analyzed gathering information from different magnitude representations including the modulus ($G^* = G' + iG''$), the compliance ($J^* = 1/G^* = J' - iJ''$) and the viscosity ($\eta^* = G^*/i\omega = \eta' - i\eta''$). Although the information contained in different representations is the same, some representation can either underline or obscure the presence of different processes due to changes in relative intensity or more pronounced power law changes with frequency. Complex viscosity representation, for example, has proven to be particularly appropriate to highlight and characterize the non simple flow behavior of alcohols[2–4].

## II. ANALYSIS OF THE RELAXATION CURVES

Phenomenological description of BDS and shear data was accomplished assuming two different contributions for the main relaxation observed in the form of of Havriliak- Negami (HN) functions, i.e.

$$F^*(\omega) = \sum_k \frac{A_k}{(1 + (i\omega\tau_k)^a)^b}. \quad (1)$$

In the case of BDS measurements we followed the same approach used in our previous works, and fitted the derivative of $\epsilon'(\omega)$ to the real part of the derivative of equation 1 (see[1] for additional details). Due to the large overlapping and disparate intensities of the two components within the main dielectric peak, the timescale of the faster component and the widths of the faster and slower components are coupled parameters preventing an accurate determination of the faster component dynamics. To be consistent with the assumption of a quasi-universal shape for the slow component we limited the shape of the slower component to HN functions closely equivalent to Kolrausch-Williamns-Watts decays in the time domain[5], i.e. those with $b = 1 - 0.8121 * (1 - a)^{0.387}$, and leading to a $\beta_{KWW}$ value close to 0.5 through the relation $\beta_{KWW}^{1.23} = a \cdot b$. The complete description of BDS data also included a third contribution accounting for the faster secondary relaxation which is not discussed in the manuscript.

Shear magnitudes $\eta''(\omega)$ and derivative of $J'(\omega)$ were directly fitted to $Im[F^*(\omega)]$. In the first instance, we also tried to fit the derivative of $J'(\omega)$ by the derivative of equation 1 in the same philosophy as dielectric data but fittings could not properly describe data.

## III. COMPARISON OF VARIOUS CHARACTERISTIC TIMES

Figure S2 shows the characteristics times at the maxima, $\tau_{max} = 1/\omega_{max} = 1/2\pi f$, of the various individual components obtained by the data analysis described above (squares and circles for slow and fast components respectively; filled symbols stand for shear data and empty symbols for dielectric data). Due to the large overlapping and disparate intensities of the two components in the dielectric data different fittings could equally describe data with slightly different values for the intensity and characteristic timescales for the slow component. Different open circles for a given temperature represent the values obtained for a set of independent fittings representing the uncertainty in timescales determination by this method. According to the qualitative analysis of the lineshape in figure S1 the outcome of the fitting procedure also shows that the separation between the characteristic times of the various components decreases at the lowest temperatures close to the glass transition. For shear data, characteristic times of the various components reasonably agree for compliance and viscosity representations. Regarding the decomposition of the dielectric signal, the fast dielectric component agrees fairly well with those obtained from shear data. The low frequency dielectric component however, is around 0.5 decades slower than the slower shear component.

Regarding comparison with data in the literature the work of Moch et al. did not contemplate the multimodal character of the shear response of TBP. As a consequence, timescales extracted from shear compliance and viscosimetry data were fitted together under a single Vogel Fulcher Tamman equation and showed different temperature dependence from dielectric times (figure S2 in reference[6]). As shown in the manuscript, shear compliance measurements underline the slower component while viscosity representation emphasizes the faster one. As a consequence, in agreement with our results and data analysis shear compliance times by Moch et al. (yellow crossed squares) closely follow slow component characteristic times while viscosimetry data (yellow diamonds) reflect the faster one.

The characteristic times obtained from dielectric data in this work agree well with the dielectric data obtained by Pabst et al. (extracted from maxima positions in figure 1 of reference[7]) within experimental uncertainty. We extracted timescales from maxima positions of DLS data in figure 1 of reference[7] an include them in figure S2. DLS times are close to the faster component identified in this work for the lowest temperatures reported but

at higher temperatures locate in between the slower and faster components identified in this work.

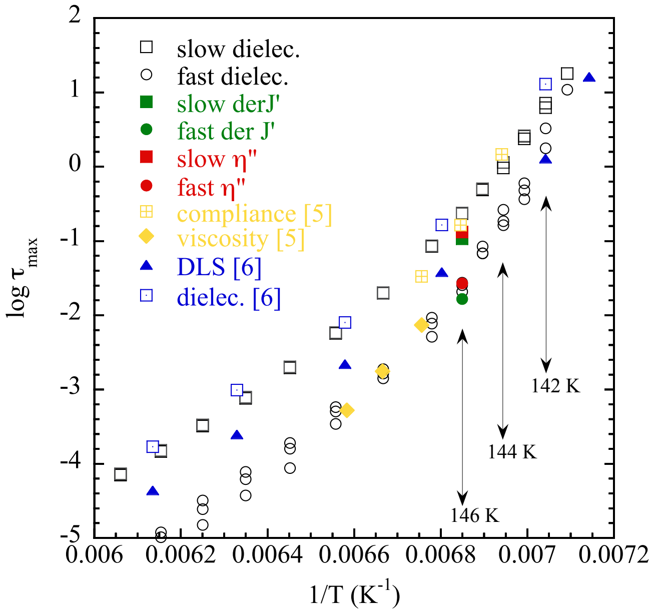


FIG. 3: Characteristic timescales for various components and techniques. For data in the present manuscript squares and circles stand for slow and fast components respectively: empty symbols dielectric data; filled red symbols stand for shear viscosity data and filled green symbols for shear compliance. Yellow symbols represent shear data from reference [5], crossed squares for compliance and diamonds for viscosimetry. Blue symbols represent data from reference [6], DLS -triangles- and dielectric -dotted squares-.

**Sample CRediT author statement**

**S. Arrese-Igor** Conceptualization, Methodology, Formal analysis, Investigation, Writing - Original Draft, Visualization. **A. Alegría** Data curation, Resources, Writing - Review & Editing, Supervision, Project administration, Funding acquisition. **J. Colmenero** Resources, Writing - Review & Editing, Supervision, Project administration, Funding acquisition.

**Acknowledgments**

We acknowledge the Grant PID2021-123438NB-I00 funded by MCIN/AEI /10.13039/501100011033 and by 'ERDF A way of making Europe' and grant IT1566-22 by the Basque Government.

[1] S. Arrese-Igor, A. Alegría, and J. Colmenero. Dielectric relaxation of 2ethyl-1hexanol around the glass transition by thermally stimulated depolarization currents. *J. Chem. Phys.*, **2015**, 142, 214504.

[2] S. Arrese-Igor, A. Alegría, and J. Colmenero. Multimodal character of shear viscosity response in hydrogen bonded liquids. *Phys. Chem. Chem. Phys.* **2018**, 20, 27758-27765.

[3] S. Arrese-Igor, A. Alegría, A. Arbe and J. Colmenero. Insights into the Non-exponential Behaviour of the Dielectric Debye-like Relaxation in Monoalcohols. *J. Mol. Liq.*, **2020**, doi: 10.1016/j.molliq.2020.113441.

[4] S. Arrese-Igor, A. Alegría, and J. Colmenero. Signature of hydrogen bonding association in the dielectric signal of polyalchols . *J. Mol. Liq.*, **2020**, 318, 114215.

[5] F. Alvarez, a. Alegria nad J. Colmenero. *Phys. Rev. B*, **1991**, 44, 7306.

[6] K. Moch, P. Munzner, R. Böhmer and C. Gainaru *Evidence for the Collective Nature of the Glass Transition. Phys. Rev. Lett.* **2022**, 128, 228001.

[7] F. Pabst, A. Helbling, J. Gabriel, P. Weigl and T. Blochowicz. Dipole-dipole correlations and the Debye process in the dielectric response of nonassociating glass forming liquids. *Physical Review E* **2020**, 102, 110606(R).
